# Supplementary material for: On symmetric decompositions of positive operators
Source: arXiv:1609.05060 ancillary file (2016-09-16)

# Numerical routines for Example 3.18

This file contains some computations related to Example  
3.18 in "On symmetric decompositions of positive operators"  
by Maria Jivulescu, Pasc Gavruta and Ion Nechita

```
In[64]:= T = {{1, 0}, {0, u}};  
F1 = {{0, 1}, {1, 0}} / Sqrt[2];  
F2 = {{0, I}, {-I, 0}} / Sqrt[2];  
F3 = {{u, 0}, {0, -1}} / Sqrt[1 + u^2];
```

```
In[68]:= T // MatrixForm  
F1 // MatrixForm  
F2 // MatrixForm  
F3 // MatrixForm
```

Out[68]//MatrixForm=

$$\begin{pmatrix} 1 & 0 \\ 0 & u \end{pmatrix}$$

Out[69]//MatrixForm=

$$\begin{pmatrix} 0 & \frac{1}{\sqrt{2}} \\ \frac{1}{\sqrt{2}} & 0 \end{pmatrix}$$

Out[70]//MatrixForm=

$$\begin{pmatrix} 0 & \frac{i}{\sqrt{2}} \\ -\frac{i}{\sqrt{2}} & 0 \end{pmatrix}$$

Out[71]//MatrixForm=

$$\begin{pmatrix} \frac{u}{\sqrt{1+u^2}} & 0 \\ 0 & -\frac{1}{\sqrt{1+u^2}} \end{pmatrix}$$

We check the fact that F1, F2, F3 form a basis of the orthogonal space to T

```

In[72]:= Tr[F1.F1]
Tr[F2.F2]
Tr[F3.F3] // Simplify
Tr[F1.F2]
Tr[F1.F3]
Tr[F2.F3]
Tr[F1.T]
Tr[F2.T]
Tr[F3.T]

```

Out[72]= 1

Out[73]= 1

Out[74]= 1

Out[75]= 0

Out[76]= 0

Out[77]= 0

Out[78]= 0

Out[79]= 0

Out[80]= 0

**We compute the operators R1, R2, R3, R4, as well as their eigenvalues**

```

In[81]:= F = F1 + F2 + F3;
R1 = F - 6 * F1;
R2 = F - 6 * F2;
R3 = F - 6 * F3;
R4 = 3 * F;
{μ1, ρ1} = FullSimplify[Eigenvalues[R1], u > 0]
FullSimplify[Eigenvalues[R2], u > 0]
{μ2, ρ2} = FullSimplify[Eigenvalues[R3], u > 0]
{μ3, ρ3} = FullSimplify[Eigenvalues[R4], u > 0]
μ1 = -μ1;
μ2 = -μ2;
μ3 = -μ3;

```

$$\text{Out[86]} = \left\{ \frac{-1 + u - \sqrt{53 + u(2 + 53u)}}{2\sqrt{1 + u^2}}, \frac{-1 + u + \sqrt{53 + u(2 + 53u)}}{2\sqrt{1 + u^2}} \right\}$$

$$\text{Out[87]} = \left\{ \frac{-1 + u - \sqrt{53 + u(2 + 53u)}}{2\sqrt{1 + u^2}}, \frac{-1 + u + \sqrt{53 + u(2 + 53u)}}{2\sqrt{1 + u^2}} \right\}$$

$$\text{Out[88]} = \left\{ -\frac{-5 + 5u + \sqrt{29 + u(50 + 29u)}}{2\sqrt{1 + u^2}}, \frac{5 - 5u + \sqrt{29 + u(50 + 29u)}}{2\sqrt{1 + u^2}} \right\}$$

$$\text{Out[89]} = \left\{ -\frac{3(1 - u + \sqrt{5 + u(2 + 5u)})}{2\sqrt{1 + u^2}}, \frac{3(-1 + u + \sqrt{5 + u(2 + 5u)})}{2\sqrt{1 + u^2}} \right\}$$

**We check the inequality  $\mu_2 > \mu_1 > \mu_3$**

`Plot[ $\mu_2 - \mu_1$ , {u, 0, 10}]`

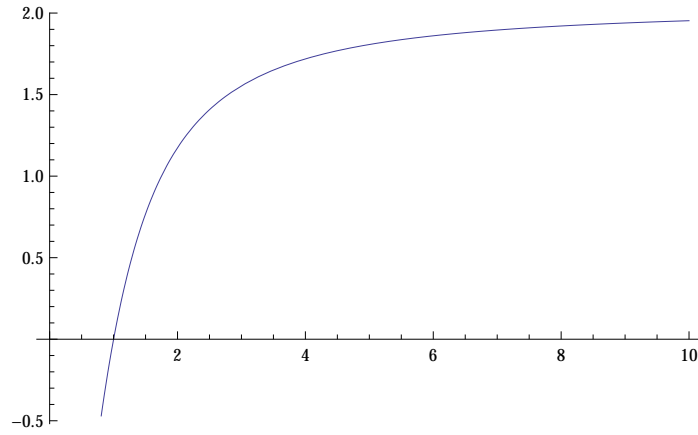

`Plot[ $\mu_1 - \mu_3$ , {u, 0, 10}]`

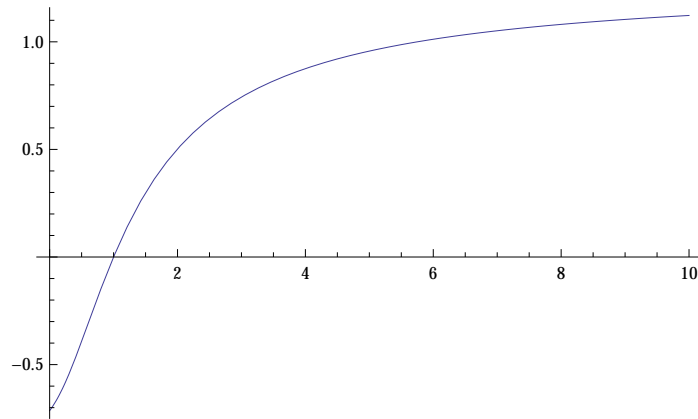

**We compute the decomposition operators E1, E2, E3, E4, as well as their eigenvalues**

```
In[110]:= E1 = T / 4 + x * R1;
E2 = T / 4 + x * R2;
E3 = T / 4 + x * R3;
E4 = T / 4 + x * R4;
{q1, w1} = FullSimplify[Eigenvalues[E1], u > 0 && x > 0]
{q2, w2} = FullSimplify[Eigenvalues[E2], u > 0 && x > 0]
{q3, w3} = FullSimplify[Eigenvalues[E3], u > 0 && x > 0]
{q4, w4} = FullSimplify[Eigenvalues[E4], u > 0 && x > 0]
```

$$\text{Out[114]} = \left\{ \frac{1}{8\sqrt{1+u^2}} \left( \sqrt{1+u^2} - 4x + u \left( \sqrt{1+u^2} + 4x \right) - \sqrt{\left( (-1+u)^2 (1+u^2) + 8\sqrt{1+u^2} x - 8u^2 \sqrt{1+u^2} x + 16(53+u(2+53u)) x^2 \right)} \right), \right. \\ \left. \frac{1}{8\sqrt{1+u^2}} \left( \sqrt{1+u^2} - 4x + u \left( \sqrt{1+u^2} + 4x \right) + \sqrt{\left( (-1+u)^2 (1+u^2) + 8\sqrt{1+u^2} x - 8u^2 \sqrt{1+u^2} x + 16(53+u(2+53u)) x^2 \right)} \right) \right\}$$

$$\begin{aligned}
\text{Out}[115] = & \left\{ \frac{1}{8\sqrt{1+u^2}} \left( \sqrt{1+u^2} - 4x + u \left( \sqrt{1+u^2} + 4x \right) - \right. \right. \\
& \left. \sqrt{\left( (-1+u)^2 (1+u^2) + 8\sqrt{1+u^2} x - 8u^2 \sqrt{1+u^2} x + 16(53+u(2+53u)) x^2 \right)} \right), \\
& \frac{1}{8\sqrt{1+u^2}} \left( \sqrt{1+u^2} - 4x + u \left( \sqrt{1+u^2} + 4x \right) + \right. \\
& \left. \left. \sqrt{\left( (-1+u)^2 (1+u^2) + 8\sqrt{1+u^2} x - 8u^2 \sqrt{1+u^2} x + 16(53+u(2+53u)) x^2 \right)} \right) \right\} \\
\text{Out}[116] = & \left\{ \frac{1}{8\sqrt{1+u^2}} \left( \sqrt{1+u^2} + u \left( \sqrt{1+u^2} - 20x \right) + 20x - \right. \right. \\
& \left. \sqrt{\left( (-1+u)^2 (1+u^2) - 40\sqrt{1+u^2} x + 40u^2 \sqrt{1+u^2} x + 16(29+u(50+29u)) x^2 \right)} \right), \\
& \frac{1}{8\sqrt{1+u^2}} \left( \sqrt{1+u^2} + u \left( \sqrt{1+u^2} - 20x \right) + 20x + \right. \\
& \left. \left. \sqrt{\left( (-1+u)^2 (1+u^2) - 40\sqrt{1+u^2} x + 40u^2 \sqrt{1+u^2} x + 16(29+u(50+29u)) x^2 \right)} \right) \right\} \\
\text{Out}[117] = & \left\{ \frac{1}{8\sqrt{1+u^2}} \left( \sqrt{1+u^2} - 12x + u \left( \sqrt{1+u^2} + 12x \right) - \right. \right. \\
& \left. \sqrt{\left( (-1+u)^2 (1+u^2) + 24\sqrt{1+u^2} x - 24u^2 \sqrt{1+u^2} x + 144(5+u(2+5u)) x^2 \right)} \right), \\
& \frac{1}{8\sqrt{1+u^2}} \left( \sqrt{1+u^2} - 12x + u \left( \sqrt{1+u^2} + 12x \right) + \right. \\
& \left. \left. \sqrt{\left( (-1+u)^2 (1+u^2) + 24\sqrt{1+u^2} x - 24u^2 \sqrt{1+u^2} x + 144(5+u(2+5u)) x^2 \right)} \right) \right\}
\end{aligned}$$

**The eigenvalue q3 is the smallest one**

```
In[137]:= Plot[{q1 /. {u → uTest}, q2 /. {u → uTest}, q3 /. {u → uTest}, q4 /. {u → uTest}},
  {x, 1, 10}, PlotLegends → LineLegend["Expressions"]]
```

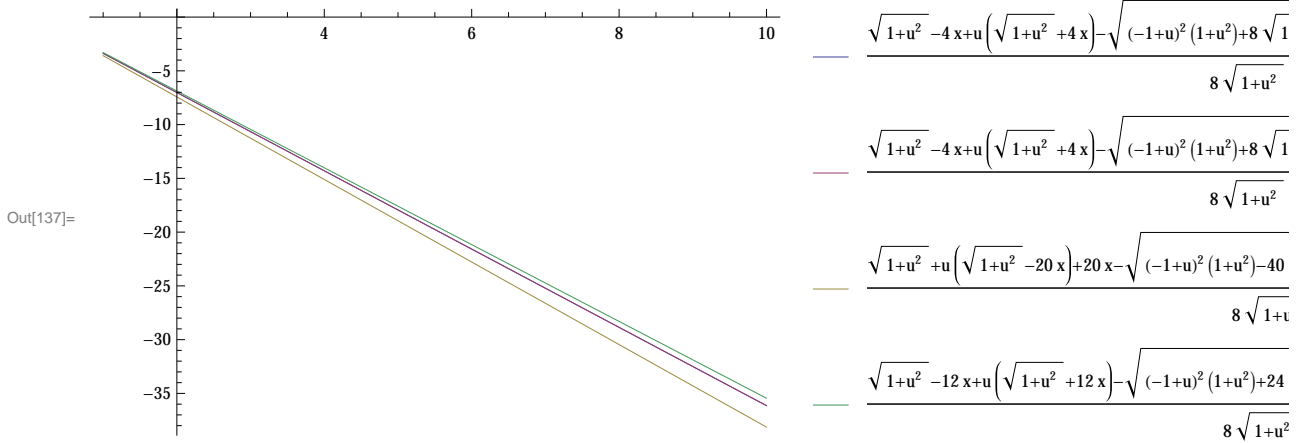

**We find the largest value of x for which the operators E are still PSD**

```
In[141]:= xoptsol = Solve[q3 == 0, x]
Plot[{x /. xoptsol[[1]], x /. xoptsol[[2]]}, {u, 1, 10}]
```

Out[141]=

$$\left\{ \left\{ x \rightarrow \left( -\sqrt{1+u^2} \left( -20 + 20u^2 \right) - 4\sqrt{25+4u+75u^2+8u^3+75u^4+4u^5+25u^6} \right) / \left( 2 \left( 16 + 400u + 16u^2 \right) \right) \right\}, \right. \\ \left. \left\{ x \rightarrow \left( -\sqrt{1+u^2} \left( -20 + 20u^2 \right) + 4\sqrt{25+4u+75u^2+8u^3+75u^4+4u^5+25u^6} \right) / \left( 2 \left( 16 + 400u + 16u^2 \right) \right) \right\} \right\}$$

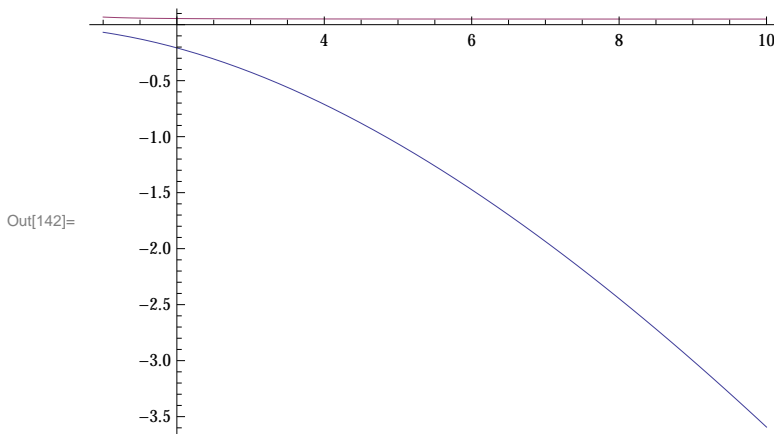

```
In[180]:= xopt = x /. xoptsol[[2]]
aopt = FullSimplify[(1 + u^2) / 16 + xopt^2 * 3 * 3^2, u > 1]
```

Out[180]=

$$\left( -\sqrt{1+u^2} \left( -20 + 20u^2 \right) + 4\sqrt{25+4u+75u^2+8u^3+75u^4+4u^5+25u^6} \right) / \left( 2 \left( 16 + 400u + 16u^2 \right) \right)$$

Out[181]=

$$\frac{1}{16} \left( 1 + u^2 + \left( 27 \left( 5\sqrt{1+u^2} - 5u^2\sqrt{1+u^2} + (1+u^2)\sqrt{25+u(4+25u)} \right)^2 \right) / \left( 4(1+u(25+u))^2 \right) \right)$$

**We check the positivity of Ei**

```
In[223]:= Plot[{q1 /. {x -> xopt}, q2 /. {x -> xopt},
               q3 /. {x -> xopt}, q4 /. {x -> xopt}}, {u, 1, 10}]
```

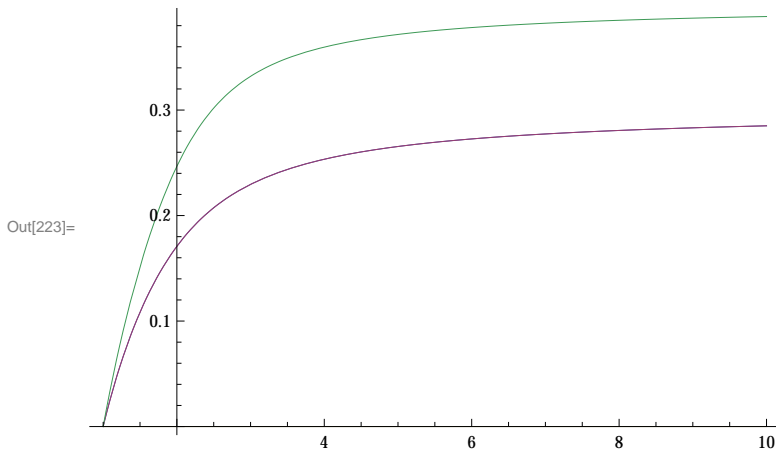

**The lower bound for x is taken from Proposition 3.8**

```
In[224]:= xLB = 1 / μ2 / 4;
FullSimplify[xLB, u > 1]
aLB = (1 + u^2) / 16 + xLB^2 * 3 * 3^2;
FullSimplify[aLB, u > 1]
aLB
```

Out[225]=

$$\frac{\sqrt{1+u^2}}{2 \left( -5 + 5u + \sqrt{29+u(50+29u)} \right)}$$

Out[227]=

$$\frac{1}{16} (1+u^2) \left( 1 + \frac{108}{\left( -5 + 5u + \sqrt{29+u(50+29u)} \right)^2} \right)$$

Out[228]=

$$\frac{1}{16} (1+u^2) + \frac{27 (1+u^2)}{4 \left( -5 + 5u + \sqrt{29+u(50+29u)} \right)^2}$$

**The upper bound for x is taken from Proposition 3.15**

```

aUB = (1 + u^2)^2 / 16;
Plot[aUB - aLB, {u, 1, 10}]
FullSimplify[aopt - aLB, u > 1]

```

$$\text{Out[204]} = \frac{1}{16} (1 + u^2) \left( 1 + \frac{108}{(-5 + 5u + \sqrt{29 + u(50 + 29u)})^2} \right)$$

$$\text{Out[205]} = \frac{1}{16} (1 + u^2) + \frac{27 (1 + u^2)}{4 (-5 + 5u + \sqrt{29 + u(50 + 29u)})^2}$$

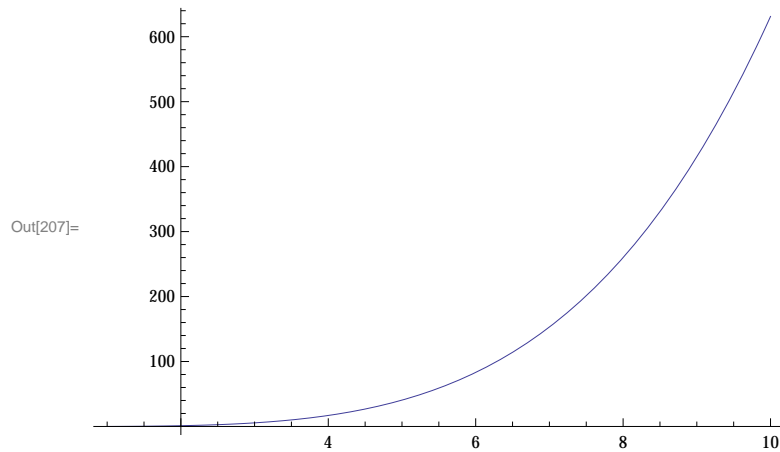

$$\text{Out[208]} = \frac{1}{16} \left( \left( 27 \left( 5 \sqrt{1 + u^2} - 5 u^2 \sqrt{1 + u^2} + (1 + u^2) \sqrt{25 + u(4 + 25u)} \right)^2 \right) / (4 (1 + u(25 + u))^2) - \frac{108 (1 + u^2)}{(-5 + 5u + \sqrt{29 + u(50 + 29u)})^2} \right)$$

**We check to see that the bounds are satisfied;  
note how the lower bound is much closer to the optimal value**

```
In[211]:= Plot[aopt - aLB, {u, 1, 10}, AxesOrigin -> {1, 0}]
Plot[aUB - aopt, {u, 1, 10}, AxesOrigin -> {1, 0}]
```

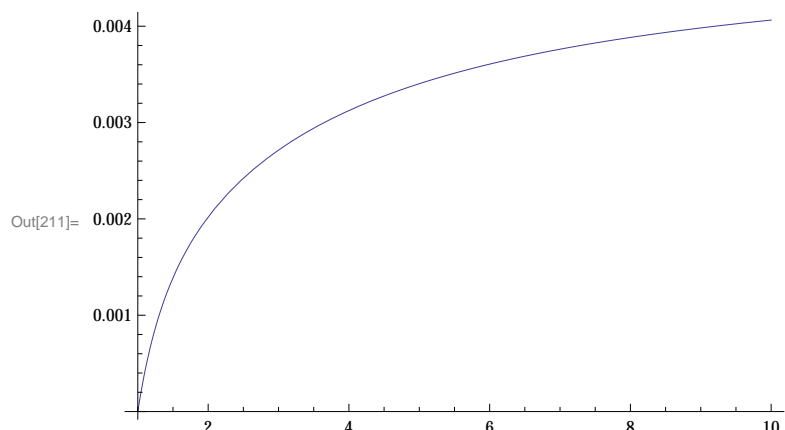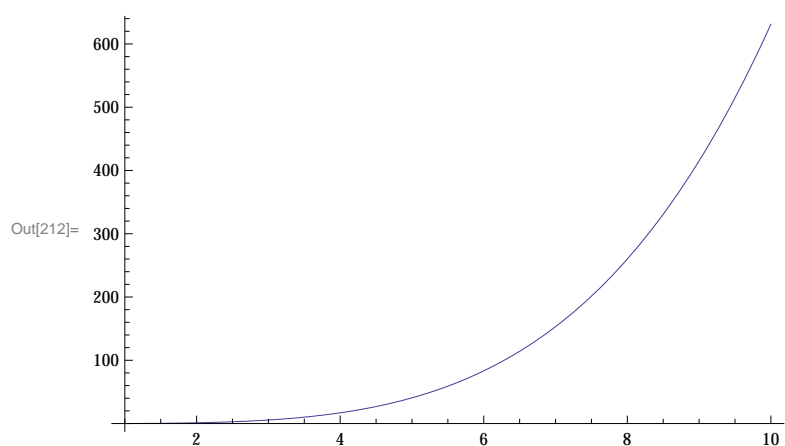

```
In[222]:= Series[aopt - aLB, {u, 1, 5}]
```

$$\begin{aligned} \text{Out[222]} = & \left( \frac{1}{8} - \frac{5}{24\sqrt{3}} \right) (u-1) + \left( \frac{25}{144} - \frac{5}{16\sqrt{3}} \right) (u-1)^2 + \left( \frac{25}{216} - \frac{475}{2592\sqrt{3}} \right) (u-1)^3 + \\ & \left( \frac{125}{7776} - \frac{265}{5184\sqrt{3}} \right) (u-1)^4 + \left( \frac{25}{3888} + \frac{10225}{559872\sqrt{3}} \right) (u-1)^5 + O[u-1]^6 \end{aligned}$$

**The lower bound is never far from the optimal value**

```
In[216]:= Limit[aopt - aLB, u -> Infinity]
% // N
```

$$\text{Out[216]} = \frac{27}{800} (-673 + 125\sqrt{29})$$

Out[217]= 0.00491403

```
In[193]:= FullSimplify[aUB - aLB, u > 1]
```

$$\text{Out[193]} = \frac{1}{16} \left( -1 - u^2 + (1 + u^2)^2 - \frac{108(1 + u^2)}{(-5 + 5u + \sqrt{29 + u(50 + 29u)})^2} \right)$$



```
In[196]:= Plot[{aopt, aLB, aUB}, {u, 1, 3}, AxesLabel → {u, a},
  PlotRangePadding → 0, AxesOrigin → {1, 0}]
```

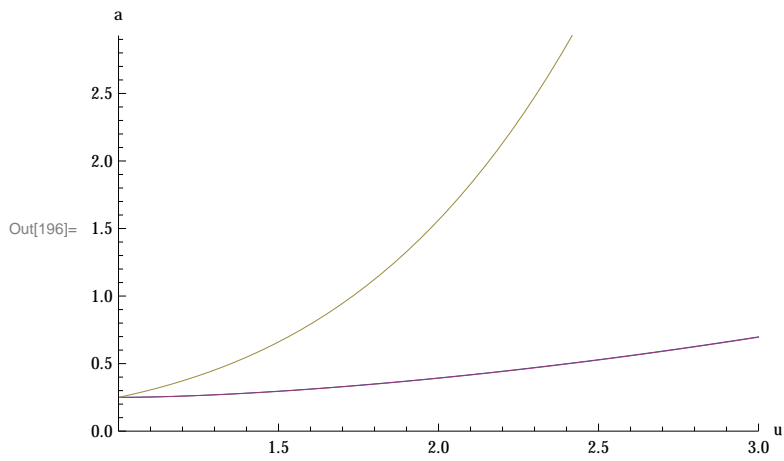

```
In[229]:= Plot[{aLB, aUB}, {u, 1, 3}, AxesLabel → {u, a},
  PlotRangePadding → 0, AxesOrigin → {1, 0}]
```

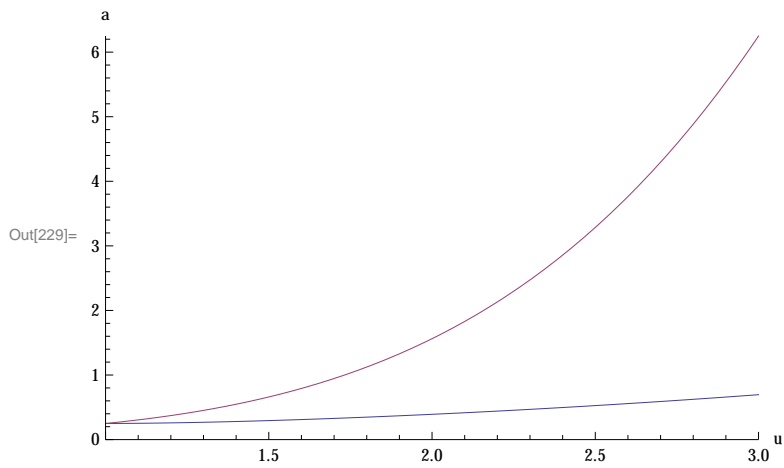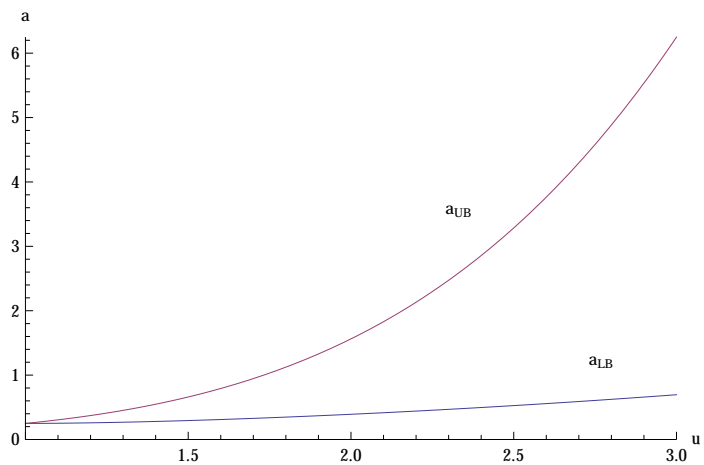

Supplement: Supplementary file 1 [file example-T-2-4.pdf]
